# Supplementary material for: OneFormer: One Transformer to Rule Universal Image Segmentation
Source: arXiv:2211.06220 source file (2022-12-27)
Supplement: Supplementary file 1 [file cityscapes.tex]

\begin{tabular}{ll|cc|cc|cccc}
   \textbf{Method} & \textbf{Backbone} & \#\textbf{Params} & \#\textbf{Queries} & \textbf{Crop Size} & \begin{tabular}{@{}c@{}} \textbf{Iters} \end{tabular} & \textbf{PQ} & \textbf{AP} & \begin{tabular}{@{}c@{}} \textbf{mIoU} \\ (s.s.) \end{tabular} & \begin{tabular}{@{}c@{}} \textbf{mIoU} \\ (m.s.) \end{tabular} \\

    \midrule
    \midrule
    \multicolumn{7}{l}{\textit{\textbf{Individual Training}}}\\
    \midrule
    \midrule
    
    \begin{tabular}{@{}l@{}}Mask2Former~\cite{mask2former} \end{tabular} & Swin-T~\cite{swin-T} & 47M & 100 & $512\!\times\!1024$ & 90k  & \begin{tabular}{@{}c@{}} 63.9  \end{tabular} & \begin{tabular}{@{}c@{}} 39.7 \end{tabular} & \begin{tabular}{@{}c@{}} 82.1 \end{tabular} & 83.0 \\
    
    \begin{tabular}{@{}l@{}}Mask2Former~\cite{mask2former} \end{tabular} & Swin-S~\cite{swin-T} & 69M & 100 & $512\!\times\!1024$ & 90k  & \begin{tabular}{@{}c@{}} 64.8  \end{tabular} & \begin{tabular}{@{}c@{}} 41.8 \end{tabular} & \begin{tabular}{@{}c@{}} 82.6 \end{tabular} & 83.6 \\
    
    \begin{tabular}{@{}l@{}}Mask2Former~\cite{mask2former} \end{tabular} & Swin-B$^\dag$~\cite{swin-T} & 107M & 100 & $512\!\times\!1024$ & 90k  & \begin{tabular}{@{}c@{}} 66.1  \end{tabular} & \begin{tabular}{@{}c@{}} 42.0 \end{tabular} & \begin{tabular}{@{}c@{}} 83.3 \end{tabular} & 84.5 \\
    
    \midrule
    \midrule
    \multicolumn{8}{l}{\textit{\textbf{Joint Training}}}\\
    \midrule
    \midrule
    
    \begin{tabular}{@{}l@{}} \textbf{\modelname} \end{tabular} & Swin-T~\cite{swin-T} & 51M & 120 & $512\!\times\!1024$ & 90k  & \begin{tabular}{@{}c@{}} 64.9  \end{tabular} & \begin{tabular}{@{}c@{}} 40.9 \end{tabular} & \begin{tabular}{@{}c@{}} 80.4 \end{tabular} & 82.1\\
    
    \begin{tabular}{@{}l@{}} \textbf{\modelname} \end{tabular} & Swin-S~\cite{swin-T} & 72M & 150 & $512\!\times\!1024$ & 90k  & \begin{tabular}{@{}c@{}} 66.0  \end{tabular} & \begin{tabular}{@{}c@{}} 43.0 \end{tabular} & \begin{tabular}{@{}c@{}} 81.6$^*$ \end{tabular} & 82.8$^*$ \\
    
    \begin{tabular}{@{}l@{}} \textbf{\modelname} \end{tabular} & Swin-B$^\dag$~\cite{swin-T} & 110M & 150 & $512\!\times\!1024$ & 90k  & \begin{tabular}{@{}c@{}} 66.3  \end{tabular} & \begin{tabular}{@{}c@{}} 44.2 \end{tabular} & \begin{tabular}{@{}c@{}} 82.6 \end{tabular} & 83.4 \\
   
    \bottomrule
    
\end{tabular}
